# Supplementary material for: Instance-dependent Noisy-label Learning with Graphical Model Based Noise-rate Estimation
Source: arXiv:2305.19486 source file (2024-07-05)
Supplement: Supplementary file 1 [file dividemix_supp.tex]

\begin{table}[t]
    \centering
    \caption{\emph{(left)} Test accuracy \% and \emph{(right)} final estimated noise rate \(\epsilon\) on CIFAR100~\cite{krizhevsky2009learning} under symmetric IIN~\cite{li2020dividemix}. Other models' results are from~\hyperref[supp:ref1]{{\textcolor{black}{[}}\textcolor{MidnightBlue}{55}\textcolor{black}{]}}~\hyperref[supp:ref2]{{\textcolor{black}{[}}\textcolor{MidnightBlue}{56}\textcolor{black}{]}}. Here, we integrate DivideMix~\cite{li2020dividemix} into our proposed model.}
    \label{table:cifar100_supp}
    \begin{subtable}[t]{0.45\linewidth}
        \centering
        % \addtolength{\tabcolsep}{-0.1em}
        \begin{tabular}{l c c}
            \toprule
            \multirow{2}{*}{\bfseries Method } & \multicolumn{2}{c}{\bfseries Noise Rates - IDN} \\
            \cmidrule{2 - 3} 
            & \textbf{0.5} & \textbf{0.9}  \\
            \midrule
            CE~\cite{yao2021instance} & 37.3 & 3.5\\
            ELR~\cite{liu2020early} & 70.2 & 20.5\\
            MOIT~\hyperref[supp:ref3]{{\textcolor{black}{[}}\textcolor{MidnightBlue}{57}\textcolor{black}{]}} & 64.6 & 36.0\\
            RRLT~\hyperref[supp:ref1]{{\textcolor{black}{[}}\textcolor{MidnightBlue}{55}\textcolor{black}{]}} & \textbf{74.8} & 29.3\\
            Sel-CL+T~\hyperref[supp:ref2]{{\textcolor{black}{[}}\textcolor{MidnightBlue}{56}\textcolor{black}{]}} & 72.4 & \textbf{48.8}\\
            \midrule
            DivideMix~\cite{li2020dividemix} & 72.1 & 29.2 \\
            \rowcolor{Gray!25}\textbf{DivideMix-Ours} & 74.2 & 30.1 \\
            \bottomrule
        \end{tabular}
    \end{subtable}
    \hfill
    % \begin{minipage}{.35\linewidth}
    %     \centering
    %     \begin{tabular}{l l l}
    %         \toprule
    %         \multirow{2}{*}{\small{\bfseries Actual Noise}} & \multicolumn{2}{c}{\small{\bfseries Estimated} \(\epsilon\)} \\
    %         \cmidrule{2 - 3} 
    %         & \tiny{\textbf{DivideMix}} & \tiny{\textbf{InstanceGM}} \\
    %         \midrule
    %         \textbf{0.2} & 0.18 & 0.32\\
    %         \textbf{0.3} & 0.34 & 0.37\\
    %         \textbf{0.4} & 0.47 & 0.42\\
    %         \textbf{0.5} & 0.53 & 0.47\\
    %         \bottomrule
    %     \end{tabular}
    % \end{minipage}
    % \begin{subtable}[t]{.4\linewidth}
    % \centering
    %  % \resizebox{\linewidth}{!}{
    %  \begin{tabular}{c c c}
    %     \toprule
    %     \multirow{2}{*}{\bfseries \shortstack{Actual\\Noise}} & \multicolumn{2}{c}{\bfseries Estimated noise rate} \\
    %     \cmidrule{2 - 3} 
    %     & \textbf{DivideMix} & \textbf{InstanceGM} \\
    %     \midrule
    %     0.2 & 0.18 & 0.32\\
    %     0.3 & 0.34 & 0.37\\
    %     0.4 & 0.47 & 0.42\\
    %     0.5 & 0.53 & 0.47\\
    %     \bottomrule
    % \end{tabular}
    % % }
% \end{subtable}
\begin{subtable}[t]{.45\linewidth}
        \centering
        % \addtolength{\tabcolsep}{-0.1em}
        \begin{tabular}{l c c}
            \toprule
            \multicolumn{3}{l}{\bfseries Estimated noise rates} \\
            \midrule
            \multirow{2}{*}{\bfseries Method} & \multicolumn{2}{c}{\bfseries Actual noise rate} \\
            \cmidrule{2-3}
            & \bfseries 0.5 & \bfseries 0.9\\
            \midrule
            DivideMix & 0.39 & 0.72  \\
            \bottomrule
        \end{tabular}
    \end{subtable}

\end{table}
