# Supplementary material for: Instance-dependent Noisy-label Learning with Graphical Model Based Noise-rate Estimation
Source: arXiv:2305.19486 source file (2024-07-05)
Supplement: Supplementary file 2 [file clothing_supp.tex]

\begin{table}[t]
        \centering
        \caption{Test accuracy (\%) of competing methods, and final estimated noise rate $\epsilon$ on Clothing1M~\cite{xiao2015learning}.
        Also, we have not considered competing models that rely on a clean set whilst training.
        We integrate DivideMix~\cite{li2020dividemix}, SSR~\cite{feng2021ssr} and CC~\cite{zhao2022centrality} into our model. DivdeMix~\cite{li2020dividemix} and CC~\cite{zhao2022centrality} show the mentioned results in their respective work. DivideMix-\textit{reproduced}~\cite{li2020dividemix} and CC-\textit{reproduced}~\cite{zhao2022centrality} shows the locally reproduced results. Our results are within \(1\%\) of the accuracy of the top approaches.}
        \label{table:clothing1M_supp}
        \begin{tabular}{l c c}
            \toprule
            \bfseries Method & \bfseries Test accuracy (\%) & \bfseries Estimated noise rate \\
            \midrule
            % Nested-CoTeaching~\cite{chen2021boosting} & 74.90\\
            % CC~\cite{zhao2022centrality} & 75.40\\
            % MLC~\cite{zheng2021meta} & 75.78\\
            ELR+ with C2D~\cite{zheltonozhskii2022contrast} & 74.58\\
            SSR~\cite{feng2021ssr} (class-balance) & 74.91\\
            AugDesc~\cite{nishi2021augmentation} & 75.11\\
            Jigsaw-ViT~\cite{chen2023jigsaw} & \textbf{75.40}\\
            % DivideMix~\cite{li2020dividemix} & \textbf{74.76}\\
            \hline
            DivideMix~\cite{li2020dividemix} & 74.76\\
            DivideMix~\cite{li2020dividemix}-\textit{reproduced} & 74.32\\
            \rowcolor{Gray!25}\textbf{DivideMix-Ours} & 74.41 & 0.41\\
            % AugDesc-WAW~\cite{nishi2021augmentation} & 74.72\\
            % AugDesc-WAW-Ours & 73.80 & 0.40\\
            \hline
            SSR (class-imbalance)~\cite{feng2021ssr} & 74.12 \\
            \rowcolor{Gray!25}\textbf{SSR-Ours}& 74.20 & 0.42\\
            \hline
            CC~\cite{zhao2022centrality} & 75.40\\
            CC~\cite{feng2021ssr}-\textit{reproduced} & 75.24 \\
            \rowcolor{Gray!25}\textbf{CC-Ours}& 75.31 & 0.41\\
            \bottomrule
        \end{tabular}
\end{table}
