# Supplementary material for: Instance-dependent Noisy-label Learning with Graphical Model Based Noise-rate Estimation
Source: arXiv:2305.19486 source file (2024-07-05)
Supplement: Supplementary file 5 [file ssr_supp.tex]

\begin{table}[ht]
    \centering
    \caption{Test accuracy (\(\%\)) of baseline SSR~\cite{feng2021ssr} and our approach with SSR~\cite{feng2021ssr} on CIFAR100~\cite{krizhevsky2009learning} at \(0.5\) IDN~\cite{xia2020part}. Both results are locally reproduced by us and we also show our approach's final estimated noise rate.}
    \label{tab:ssr_supp}
    \begin{tabular}{l c c}
            \toprule
            \textbf{Method} & \textbf{Test Accuracy} & \textbf{Noise Estimation} \\
            \midrule
            SSR~\cite{feng2021ssr} & 75.8 & \\
            \rowcolor{Gray!25}\textbf{SSR-Ours} & 76.9 & 0.47 \\
            \bottomrule
        \end{tabular}
\end{table}
